# Supplementary material for: Gradient Reweighting: Towards Imbalanced Class-Incremental Learning
Source: arXiv:2402.18528 source file (2024-03-29)
Supplement: Supplementary file 1 [file X_suppl.tex]

\clearpage
\setcounter{page}{1}
\maketitlesupplementary

% This phenomenon also challenges another commonly used strategy of maintaining a fixed total number of exemplars~\cite{EEIL} regardless of class distribution, which can inadvertently perpetuate the existing imbalance by allocating more memory to head classes. This oversight in highlights the need for future approaches that take the data imbalance into account, ensuring a more balanced and fair memory allocation across all classes. 

% \section*{Table of Contents}
%     \textbf{Section~\ref{supplsec: method}: Extended Illustration of Methodology}
%         \begin{itemize}
%             \item Regularized Softmax Cross-entropy
%             \item Imbalanced Catestrophic Forgetting
%         \end{itemize}
%     \textbf{Section~\ref{supplsec: setup}: Detailed Experimental Setup}
%         \begin{itemize}
%             \item Evaluation Metrics and Training Details
%             \item Exemplar Selection
%             \item The 2-Stage~\cite{liu2022long} Implementation
%         \end{itemize}
%     \textbf{Section~\ref{supplsec: results}: Additional Experimental Results}
%         \begin{itemize}
%             \item Results for Imbalanced CIL 
%             \begin{itemize}
%                 \item ImageNet-LT with 1,000 classes 
%                 \item \textit{Ordered} Long-Tailed CIL 
%                 \item Fixed Memory Exploration
%                 \item Tuning of Hyper-parameters
%             \end{itemize}
%             % \item Results for Imbalanced CIL in Online Scenario
%             \item Results for Conventional CIL 

%         \end{itemize}
% \textbf{\red{Code is available in the Zip file}}

\section{Extended Illustration of Methodology}
\label{supplsec: method}
The objective of our proposed gradient reweighting approach, as detailed in Section~\ref{sec:method}, is to mitigate bias in the fully connected (FC) layer during the CIL. This goal aligns with the motivations in previous works such as~\cite{BiC, mainatining}. However, our proposed strategy differs significantly where instead of implementing post-hoc corrections as in \cite{BiC, mainatining}, we propose to directly adjust the gradient updates during the learning phase, aiming to address the bias issue from the source. Furthermore, our approach demonstrates the flexibility in CIL by effectively addressing both intra-phase and inter-phase imbalances. This sets our method apart from existing strategies that predominantly target inter-phase issues, thus limiting the applicability in real-world scenarios characterized by non-uniform data distributions. 

Algorithm~\ref{alg:gr} illustrates the entire procedure to learn a new task $\mathcal{T}^t$. 

% algorithm block -----------------

\begin{algorithm}[t]
\caption{Gradient Reweighting}\label{alg:gr}
\begin{small} 
    \hspace*{0.02in} {\bf Input:}
    A new tasks: $\mathcal{T}^t$\\
    \hspace*{0.02in} {\bf Require:} 
    CIL model $\mathcal{M}^{t-1}(f_\theta, W)$, learning rate $\eta$\\
\vspace{-0.35cm}
\begin{algorithmic}[1]
\State Initialize $\Phi^{j}, j\in \mathcal{Y}^{1:t}$  \Comment{accumulated gradients}
\For{i = 1, 2, ... } \Comment{iteration index}
\State $\Phi^{j}_i \leftarrow \Phi^{j}_i +  ||\nabla_{\mathcal{L}_{ce}}(W_i^{j})||$
\If {$t = 1$}  \Comment{intra-phase gradient reweighting}
\State $\alpha_i^j \leftarrow \underset{m \in \mathcal{Y}^t}{\textit{min}}\Phi^m_i/\Phi^{j}_i  $ \Comment{class balance ratio}
\State $W_{i+1}^{j} \leftarrow W_i^{j} - \eta \alpha^{j}_i \nabla_{\mathcal{L}_{ce}}(W_i^{j}) $ \Comment{\textit{back prop}}
\Else \Comment{inter-phase decoupled gradient reweightinge}
% \State $r_i \leftarrow |\mathcal{Y}^{t}|\sum_{j \in \mathcal{Y}^{1:t-1}}\Phi_i^j/|\mathcal{Y}^{1:t-1}|\sum_{j \in \mathcal{Y}^{t}}\Phi_i^j$ \Comment{task balance ratio}
\State $ \alpha_i^j \leftarrow \left\{ \begin{array}{ccl}
   \underset{m \in \mathcal{Y}^{1:t-1}}{\textit{min}}\Phi^m_i/\Phi^{j}_i & j \in \mathcal{Y}^{1:t-1} \\  \underset{m \in \mathcal{Y}^{t}}{\textit{min}}\Phi^m_i/\Phi^{j}_i & j \in \mathcal{Y}^{t}
    \end{array}\right.$
\State $r_{\Phi_i} \leftarrow \frac{\overline{\Phi}_i^{j \in \mathcal{Y}^{1:t-1}}}{\overline{\Phi}_i^{j \in \mathcal{Y}^{t}}} $ \Comment{ratio of mean gradients $\overline{\Phi}$}
% \State $\alpha_i^j \leftarrow \underset{m \in \mathcal{Y}^{1:t-1}}{\textit{min}}\Phi^m_i/\Phi^{j}_i$ \Comment{learned classes}
% \State $\alpha_i^j \leftarrow \underset{m \in \mathcal{Y}^{t}}{\textit{min}}\Phi^m_i/\Phi^{j}_i$ \Comment{new classes} 
\State $ r_i^j \leftarrow \left\{ \begin{array}{ccl}
   \textit{min} \{1, \frac{1}{r_{\Phi_i}}\} & j \in \mathcal{Y}^{1:t-1} \\  \textit{min} \{1, r_{\Phi_i} \times exp( - \gamma \frac{|\mathcal{X}^{1:t-1}|}{|\mathcal{X}^{1:t}|}) \} & j \in \mathcal{Y}^{t}
    \end{array}\right.$ \Comment{task balance ratio}
\State $\beta_i \leftarrow \frac{||\alpha_i r_i \nabla_{\mathcal{L}_{ce}}(W_i)||}{||\nabla_{\mathcal{L}_{dakd}}(W_i)}||$ \Comment{loss balance ratio}
\State $W_{i+1}^{j} \leftarrow W_i^{j} - \eta (\alpha^{j}_i \nabla_{\mathcal{L}_{ce}}(W_i^{j}) + \beta_{i} \nabla_{\mathcal{L}_{kd}}(W_i^{j}))$
\EndIf
\EndFor
\State $\mathcal{M}^{t-1} \rightarrow \mathcal{M}^{t}$ \Comment{$\mathcal{T}^t$ finished}
\end{algorithmic}
\label{alg:online sampler}
\end{small}
\end{algorithm} 
% algorithm block -----------------

\subsection{Regularized Softmax Cross-entropy}
In Section~\ref{subsec: intra-phase}, we introduced the regularized softmax cross-entropy to compensate for the side effect caused by gradient reweighting during the learning phase. In this part, we further provide a detailed illustration of where the issue comes from. The main goal of gradient re-weighting is to reduce the effect of imbalanced optimization between head and tail classes by down-weighting the weight updates of head classes. However, while this adjustment helps in emphasizing tail classes, it also inadvertently leads to increased loss values for the head classes, resulting in larger gradients. Specifically, the gradient of a head class input data $(\textbf{x}_k, y_k)$ with respect to each output logit $z_j$ can be calculated as 
\begin{equation}
\label{eq: gradients}
    \frac{\partial \mathcal{L}_{ce}}{\partial z_j} = 
    \left\{ \begin{array}{ccl}
    p_{j} -1 & j = y_k \\ p_{j} & j \neq y_k
    \end{array}\right., p_j = \frac{exp(z_j)}{\sum_{m = 1}^{|\mathcal{Y}^1|}exp(z_m)}
\end{equation}
where $z_j$ is the $j$th output logit and $p_j$ is the corresponding softmax output. Attributing to the down-weight of gradients to the head class $y_k$, the output logit $z_{y_k}$ and its softmax $p_{y_k}$ decreases during the training process. Consequently, it results in an increase of the positive gradient norm $||1 - p_j||$, prompting the head class weight $W^{y_k}$ to produce a higher output logit value. Concurrently, since the total sum of softmax outputs is constrained to 1, the decrease of $p_{y_k}$ leads to the rise of the negative gradient norm $\sum_{j\neq y_k}||p_j||$, driving the tail classes weight to output even lower scores. Our method utilizes regularized softmax as in Equation~\ref{eq:r-softmax}, which effectively mitigates this side effect by adding a per-class offset $\pi_j$ to the output logit 
\begin{equation}
\label{eq:pij}
    \begin{aligned} 
    \pi_j = \left\{ \begin{array}{ccl}
   \frac{n_j}{\sum_m n_m} & t = 1 \\  \frac{\textit{min} \{n_j, n_\varepsilon\}}{\sum_m \textit{min} \{n_m, n_\varepsilon\}} & t > 1
    \end{array}\right.
    \end{aligned}
\end{equation}
where $t$ is the task index, $n_j$ is the number of training data for class $j$, and $n_\varepsilon$ denotes the exemplar budget per class. Thus, the instance-rich classes have larger $\pi_j$ with an increase of softmax output $p_j$ to compensate for the side effect of down-weighting the gradients during the training process.

\begin{figure}[t]
\begin{center}
  \includegraphics[width=1.\linewidth]{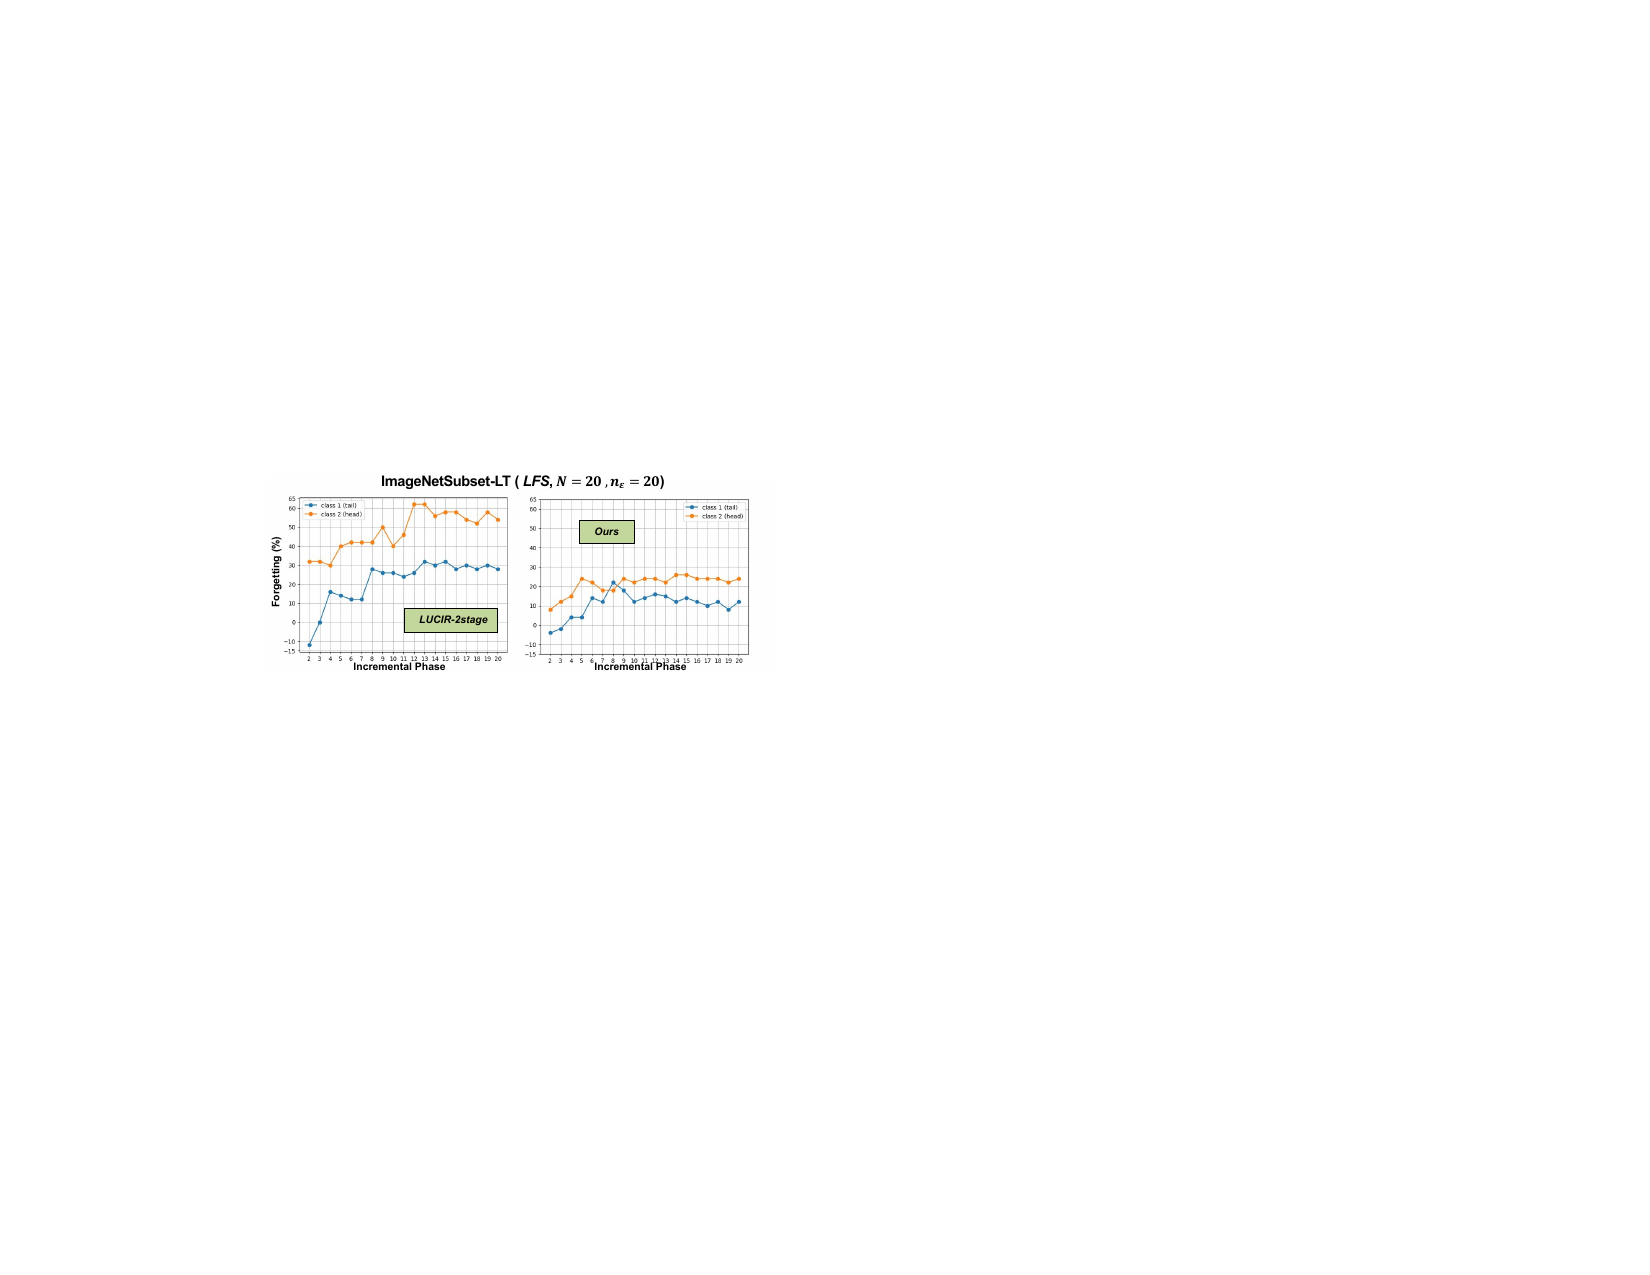}
    \caption{The forgetting rate (\%) for one selected head class and one tail class by comparing the LUCIR-2stage~\cite{rebalancing, liu2022long} and our method.   }
  \label{fig:imbalanced forgetting}
\end{center}
\end{figure}

\subsection{Imbalanced Catastrophic Forgetting}
As described in Section~\ref{sec:intro}, we argue catastrophic forgetting could also be imbalanced. In this part, we provide further illustration and also present experimental results to visualize this issue. 
In CIL, the forgetting problem mainly comes from the unavailability of old classes' training data during the learning of new classes. However, as the training data is severely imbalanced, there is a significant variance in the amount of lost training data between head and tail classes due to a fixed memory budget. During task $t$, suppose we select $n_e$ exemplars per class, thus we have $|\mathcal{X}^{j}_e| \leq n_e, \forall j \in \mathcal{Y}^{1:t-1}$ (note that some classes may contain less than $n_e$ training data). Given the class imbalance condition where $n_{j} \gg n_{k}$ for a head class $j$ and a tail class $k$, it implies that a large volume of instances from head class $j$ become unavailable in comparison to tail class $k$ in the subsequent incremental learning phases $n_{j} - n_e \gg n_{k} - n_e$. (\textit{e.g. }consider the case where a tail class $k$ has training data $n_k < n_e$, then all of the training data for class $k$ will be preserved for entire CIL.) This poses a unique challenge in CIL of imbalanced forgetting where head classes (with more training data lost) potentially suffer more performance degradation than tail classes (with less or even no training data lost). 

To visualize the imbalance forgetting issue, we perform CIL on ImageNetSubset-LT following the implementation details as described in Section~\ref{subsec: exp setup}.
Specifically, we select a tail class (class 1: 33 training images) and a head class (class 2: 1017 training images) from the initial task 1 and measure the forgetting rate $Forg = Acc_1 - Acc_i$ in each subsequent learning phase $i > 1$. $Acc$ is the accuracy on test data belonging to that specific class (\textit{i.e. } class 1 or class 2) where $Acc_i$ denotes incremental phase $i$ and $Acc_1$ is the accuracy in the initial phase when the class is firstly observed.
The result is shown in Figure~\ref{fig:imbalanced forgetting}. We observe the head class suffers a higher performance degradation compared to the tail class in LUCIR-2stage~\cite{rebalancing, liu2022long}, showing the imbalanced catastrophic forgetting phenomenon. Our method, with gradient reweighting and Distribution-Aware Knowledge distillation (DAKD) loss as illustrated in Section~\ref{sec:method}, significantly reduces the forgetting for both tail and head classes while mitigating the imbalance issue. Specifically, the DAKD effectively addresses this problem by decoupling the original knowledge distillation loss~\cite{KD} into a weighted sum of two components using a ratio $\sigma$ measured by entropy on the lost training data distribution $\textbf{s}$ with total classes $c$ as
\begin{equation}
\label{eq: entropy}
    \sigma (\textbf{s}) = \frac{-\sum_{j=1}^c v_jlog(v_j)}{log(c)} \quad v_j = \frac{s_j}{\sum_{m=1}^c s_m}
\end{equation}
% $$\sigma (\textbf{s}) = \frac{-\sum_{j=1}^c v_jlog(v_j)}{log(c)} \quad v_j = \frac{s_j}{\sum_{m=1}^c s_m} $$ 
Therefore, when $\sigma = 1$ (balanced data loss), our DAKD works equivalently as original knowledge distillation loss. When $\sigma$ decreases, it prioritizes knowledge retention from classes with greater data loss. Overall, the DAKD focuses more on preserving the performance of head classes with a greater loss of training data as well as allowing more plasticity for tail classes, enabling them to adapt more effectively to the current training data distribution. 

% in all subsequent learning phases as shown in Figure~\ref{fig:imbalanced forgetting}. 

% Besides, as we commonly store balanced exemplars for each seen class as suggested in both conventional~\cite{ICARL, EEIL} or imbalanced CIL~\cite{chrysakis2020online}, there will be a significant variance in the amount of lost training data between head and tail classes. Suppose we select $n_e$ exemplars per class, thus we have $\mathcal{X}^{y}_e = n_e, \forall y \in \mathcal{Y}^{1:N}$. Given the class imbalance condition where $n_{j} \gg n_{k}$,  it implies that a large volume of instances from head class $j$ become unavailable in comparison to tail class $k$ in the subsequent incremental learning phases $n_{j} - n_e \gg n_{k} - n_e$, which poses a unique challenge in CIL of imbalanced forgetting where head classes potentially suffer more performance degr

% In this part, I will further illustrate where this issue comes from and include a figure of experiments to show this problem in CIL. Include some illustration of DAKD and describe in detail how the ratio $\sigma$ is determined by the Entropy. 

% \subsection{Illustration of Bias Correction Effect}
% In this part, I will discuss the connection and difference between ours and existing bias correction methods, why our method work more effectively. Also, point out why we only focus on the gradients in FC layer. 

\begin{table*}[t]
    \centering
    \scalebox{1}{
    \begin{tabular}{lcccccccc}
        \hline
          \multicolumn{1}{c}{Datasets} &\multicolumn{4}{c}{\textbf{CIFAR100-LT}} & \multicolumn{4}{c}{\textbf{ ImageNetSubset-LT}} \\

          \multicolumn{1}{c}{Evaluation protocol}  & \multicolumn{2}{c}{\textit{LFS}} & \multicolumn{2}{c}{\textit{LFH}} & \multicolumn{2}{c}{\textit{LFS}} & \multicolumn{2}{c}{\textit{LFH}}\\
        \cdashline{2-9}
          \multicolumn{1}{c}{Total tasks $N$}  & 10 & 20 & 5 & 10 & 10 & 20 & 5 & 10 \\
         \hline
        iCaRL~\cite{ICARL}& 38.71 & 34.66 & 30.13 & 29.98 & 50.10 & 43.22 & 45.28 & 43.98  \\
        % EEIL~\cite{EEIL} & 31.93 & 29.42 & 34.92 & 34.13 & 32.68 & 25.64 & 40.43 & 39.65 & 17.11 & 16.83 & 24.02 & 23.30 \\
        IL2M~\cite{dualmemory}& 44.42 & 40.54 & 39.83 & 37.87 & 47.53 & 40.02 & 46.95 & 44.34 \\
        BiC~\cite{BiC} & 41.59 & 36.41 & 34.57 & 31.08 & 47.92 & 45.53 & 47.78 & 41.05 \\
        WA~\cite{mainatining} & 43.69 & 37.58 & 35.66 & 33.02 & 48.83 & 46.71 & 48.29 & 42.24   \\
        %LUCIR~\cite{rebalancing} & 28.72 & 27.79 & 34.88 & 34.07 & 34.27 & 29.72 & 45.22 & 44.98 & 23.99 & 22.38 & 32.20 & 31.11 \\
        SSIL~\cite{SSIL} & 43.25 & 35.28 & 33.90 & 23.16 & 50.62 & 41.41 & 40.00 & 41.73 \\
        % PODNet~\cite{douillard2020podnet} & 27.68 & 28.26 & 36.62 & 36.97 & 28.42 & 27.18 & 44.82 & 45.33 & 19.85 & 18.11 & 33.13 & 33.64 \\
        FOSTER~\cite{foster} &43.68 & 36.70 & 38.43 & 35.19 & 49.72 & 42.68 & 47.31 & 46.89  \\
        MAFDRC~\cite{MAFDRC} & 44.27 & 37.82 & 42.10 & 41.94 & 50.83 & 44.20 & 48.69 & 47.11  \\
        EEIL-2stage~\cite{EEIL,liu2022long} &  45.34 & \textbf{\blue{41.03}} & 39.95 & 38.85 & 50.39 & 43.57 & 50.93 & 48.37  \\
        LUCIR-2stage~\cite{rebalancing,liu2022long} & 47.83 & 36.01 & \textbf{\red{45.10}} & 43.35 & \textbf{\blue{53.47}} & 47.67 & \textbf{\blue{54.88}} & 53.38 \\
        PODNet-2stage~\cite{douillard2020podnet,liu2022long} & \textbf{\blue{48.67}} & 34.17 & 44.42 & 43.54 & 52.00 & 44.55 & 54.75 & \textbf{\red{54.21}}  \\
        FOSTER-2stage~\cite{foster,liu2022long} & 46.35 & 38.93 & 43.21 & \textbf{\red{44.18}} & 52.64 & \textbf{\blue{47.91}} & 54.26 & 53.87  \\
          \hline
        Ours & \textbf{\red{50.24}} & \textbf{\red{41.50}} & \textbf{\blue{44.87}} & \textbf{\blue{44.13}} & \textbf{\red{55.42}} & \textbf{\red{49.73}} & \textbf{\red{55.67}} & \textbf{\blue{53.95}} \\
        \hline
    \end{tabular}
    }
        \caption{Results of average accuracy (\%) for Ordered CIL on CIFAR100-LT, ImageNetSubset-LT with imbalance factor $\rho = 100$, memory budget $n_\varepsilon = 20$ evaluated under Learning From Scratch (\textit{LFS}) and Learning From Half (\textit{LFH}). \textbf{\red{Best}} and \textbf{\blue{Second Best}} results are marked. }
    \label{tab:results_ordered}
\end{table*}

\section{Detailed Experimental Setup}
\label{supplsec: setup}
\subsection{Evaluation Metrics and Training Details}
In this part, we first illustrate the evaluation metrics including the average accuracy (ACC) and forgetting rate as used in Section~\ref{sec:experiments}. Then we provide additional training details. 

\textbf{Evaluation Metrics:} The average accuracy (ACC)~\cite{GEM} considers the performance of all incremental learning phases as $$\bar{\mathcal{A}} = \frac{1}{N}\sum_{t=1}^{N}\mathcal{A}_t$$ where $\mathcal{A}_t$ is the top-1 classification accuracy after learning task $\mathcal{T}^t$ on all classes seen so far. The forgetting rate~\cite{GEM}, also known as backward transfer (BWT), measures the performance drops during CIL as calculated in
$$\bar{\mathcal{F}} = \frac{-1}{N-1}\sum_{t=1}^{N-1}\mathcal{A}_N^t - \mathcal{A}_t^t$$
where $\mathcal{A}_N^t$ refers to the classification accuracy on task $t$ after learning task $N$. In general, an expected CIL model should have higher average accuracy $\bar{\mathcal{A}}\uparrow$ as well as lower forgetting rate $\bar{\mathcal{F}}\downarrow$. 

\textbf{Training Details:} Our method is implemented with PyTorch~\cite{pytorch} based on the framework provided in~\cite{liu2022long, survey_2020}. Each experiment is run on a single NVIDIA A40 GPU with 48G memory. The class order is generated and shuffled using the identical random seed (1993) as in~\cite{liu2022long, ICARL}. Only regular data augmentation technique is included such as random flip and crop. (No AutoAugment~\cite{autoaugment} as implemented in~\cite{foster, MAFDRC}). To further ensure fair comparisons with existing work, instead of obtaining the results from the original publications, we reproduce the existing methods under the same setting three times for each experiment and report the average performance as illustrated in Section~\ref{subsec: exp setup}.

% In this part, I will illustrate the training details such as evaluation metrics, hardware, and also most importantly, how the existing methods' performance is obtained (by reproducing them instead of from the original paper). 
\subsection{Exemplar Selection}
\label{subsec-supple:exemplarselection}
In this part, we illustrate the exemplar setup used in Section~\ref{sec:experiments}. In conventional CIL, there are two widely used strategies for storing exemplars including (i) Fixed Memory (FM), and (ii) Growing Memory (GM). Specifically, the FM uses a fixed buffer size $|\mathcal{E}| = \mathcal{B}$ and split evenly for all classes seen so far thus each class contains $n_\varepsilon = \frac{\mathcal{B}}{c}$ exemplars. As more classes are encountered, $n_\varepsilon$ will decrease. On the other hand, GM uses a fixed $n_\varepsilon$ per class, thus the total exemplar size $|\mathcal{E}| = c\times n_\varepsilon$ is growing when more classes $c$ are observed. Though FM is more practical and popular in conventional CIL with balanced training data distribution, it poses two non-trivial questions in imbalanced CIL including (a) how to allocate the fixed memory size $\mathcal{B}$ to class-imbalanced data distribution, and (b) how to update the memory buffer after observing new classes.  Until now, the FM-based exemplar selection is still under-explored in imbalanced CIL (\textit{i.e. }There lacks efficient exemplar selection strategies.)

In this work, we primarily follow the setup in~\cite{liu2022long} to use GM with fixed $n_\varepsilon$. Specifically, we select up to $n_\varepsilon$ samples per class after each incremental learning phase by applying Herding algorithm~\cite{HERDING} based on the class mean. Note that for tail classes with the number of training data less than $n_\varepsilon$, we store all of their training data in the exemplar set. Therefore, the exemplar set $\mathcal{E}$ could still exhibit the class-imbalanced issue. 

Later in Section~\ref{subsec-supple:imbalanced CIL}, we also explore a variant of FM setting by using dynamic $n_\varepsilon$ in imbalanced CIL. Specifically, we set a fixed memory buffer size $\mathcal{B}$ and calculate the $n_\varepsilon = \frac{\mathcal{B}}{c}$ after learning each task. Note that this case is still different from the conventional FM setting as most classes in long-tailed distribution will have fewer training samples than \( n_\varepsilon \). However, we can ensure the total buffer size is bounded with $|\mathcal{E}| \leq \mathcal{B}$.

% In this part, I will describe the exemplar setting we used in the main paper (growing memory) and why we use it (following existing benchmark). Then I will discuss another popular setup (fixed memory) about why it may not be suitable for imbalanced CIL. 

% results on for fixed memory setup -------------------------
\begin{figure*}[t]
\begin{center}
  \includegraphics[width=1.\linewidth]{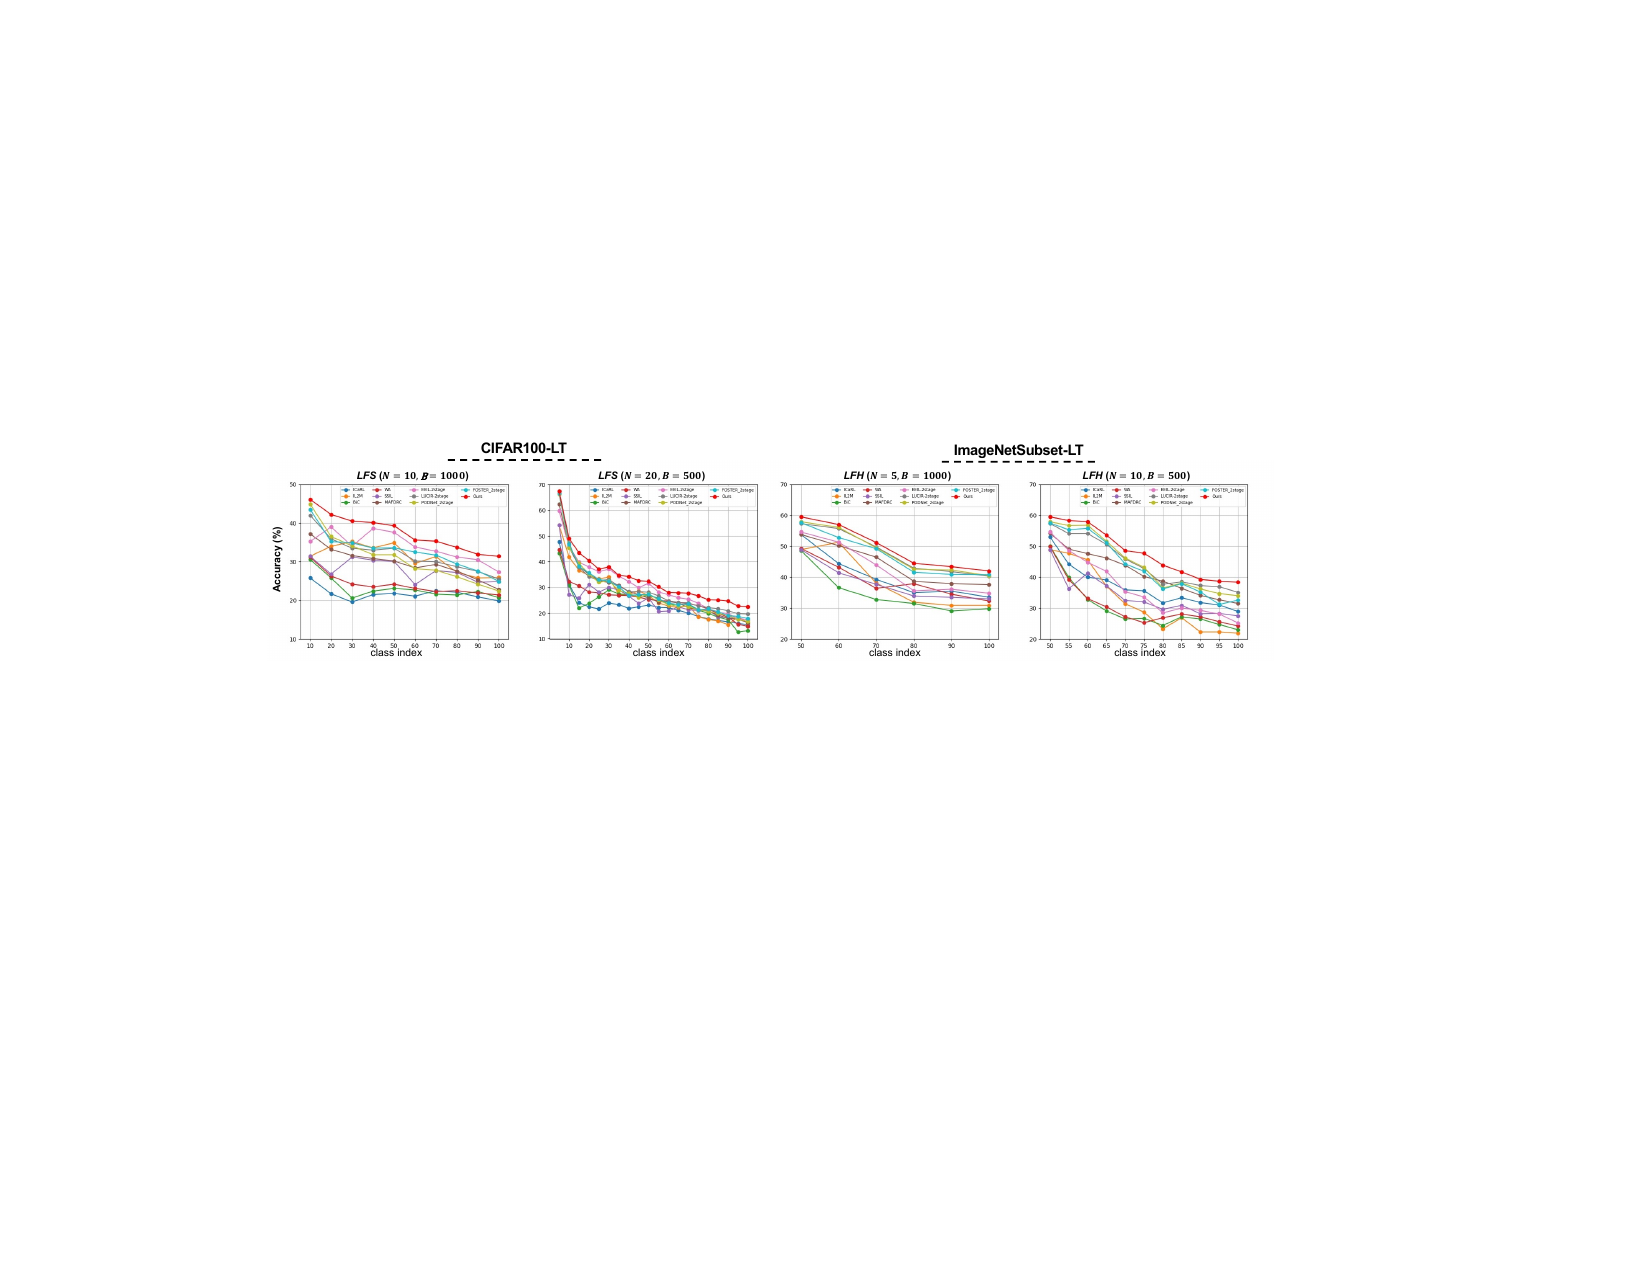}
 \caption{The classification accuracy (\%) on test data belonging to all classes seen so far at each incremental step by using the fixed memory budget $\mathcal{B} \in \{500, 1000\}$ on CIFAR100-LT and ImageNetSubset-LT with imbalance factor $\rho=100$. }
  \label{fig:fixedmemory}
\end{center}
\end{figure*}
%-----------------------------------

\subsection{The 2-Stage Implementation}
In this part, we illustrate the implementation of the 2-stage module~\cite{liu2022long} to integrate with existing conventional CIL for experiments in Section~\ref{sec:experiments}. As proposed in~\cite{liu2022long}, the 2-stage framework is structured as follows: stage-1 focuses on training the feature extractor and classifier using the entire dataset (aligned with conventional CIL training with no alternation). Subsequently, stage-2 involves the training of an additional Learnable Weight Scaling (LWS) layer using a class-balanced sampler. 

Therefore, in our implementation of the 2-stage module, each incremental phase is conducted in two steps. Initially, we perform the original method with implementation details outlined in Section~\ref{subsec: exp setup}. Following this, an additional training phase is introduced specifically to learn the Learnable Weight Scaling (LWS). During this phase, we fix parameters in the feature extractor and the classifier corresponding to the previously learned classes. The implementation details of this training phase follow the~\cite{liu2022long}, involving a fixed learning rate of $0.1$ and 30 training epochs. Note that in Table~\ref{tab:results_all}, we did not include the results for the original LUCIR~\cite{rebalancing}, EEIL~\cite{EEIL}, and PODNet~\cite{douillard2020podnet} as their 2-stage versions have been proved to be more effective for imbalanced CIL in~\cite{liu2022long}. However, we further performed the 2-stage module on FOSTER~\cite{foster} and compared it with the original results as shown in Table~\ref{tab:results_all}.

% results on imagenet-lt with 1000 classes -------------------------
\begin{figure}[t!]
\begin{center}
  \includegraphics[width=1.\linewidth]{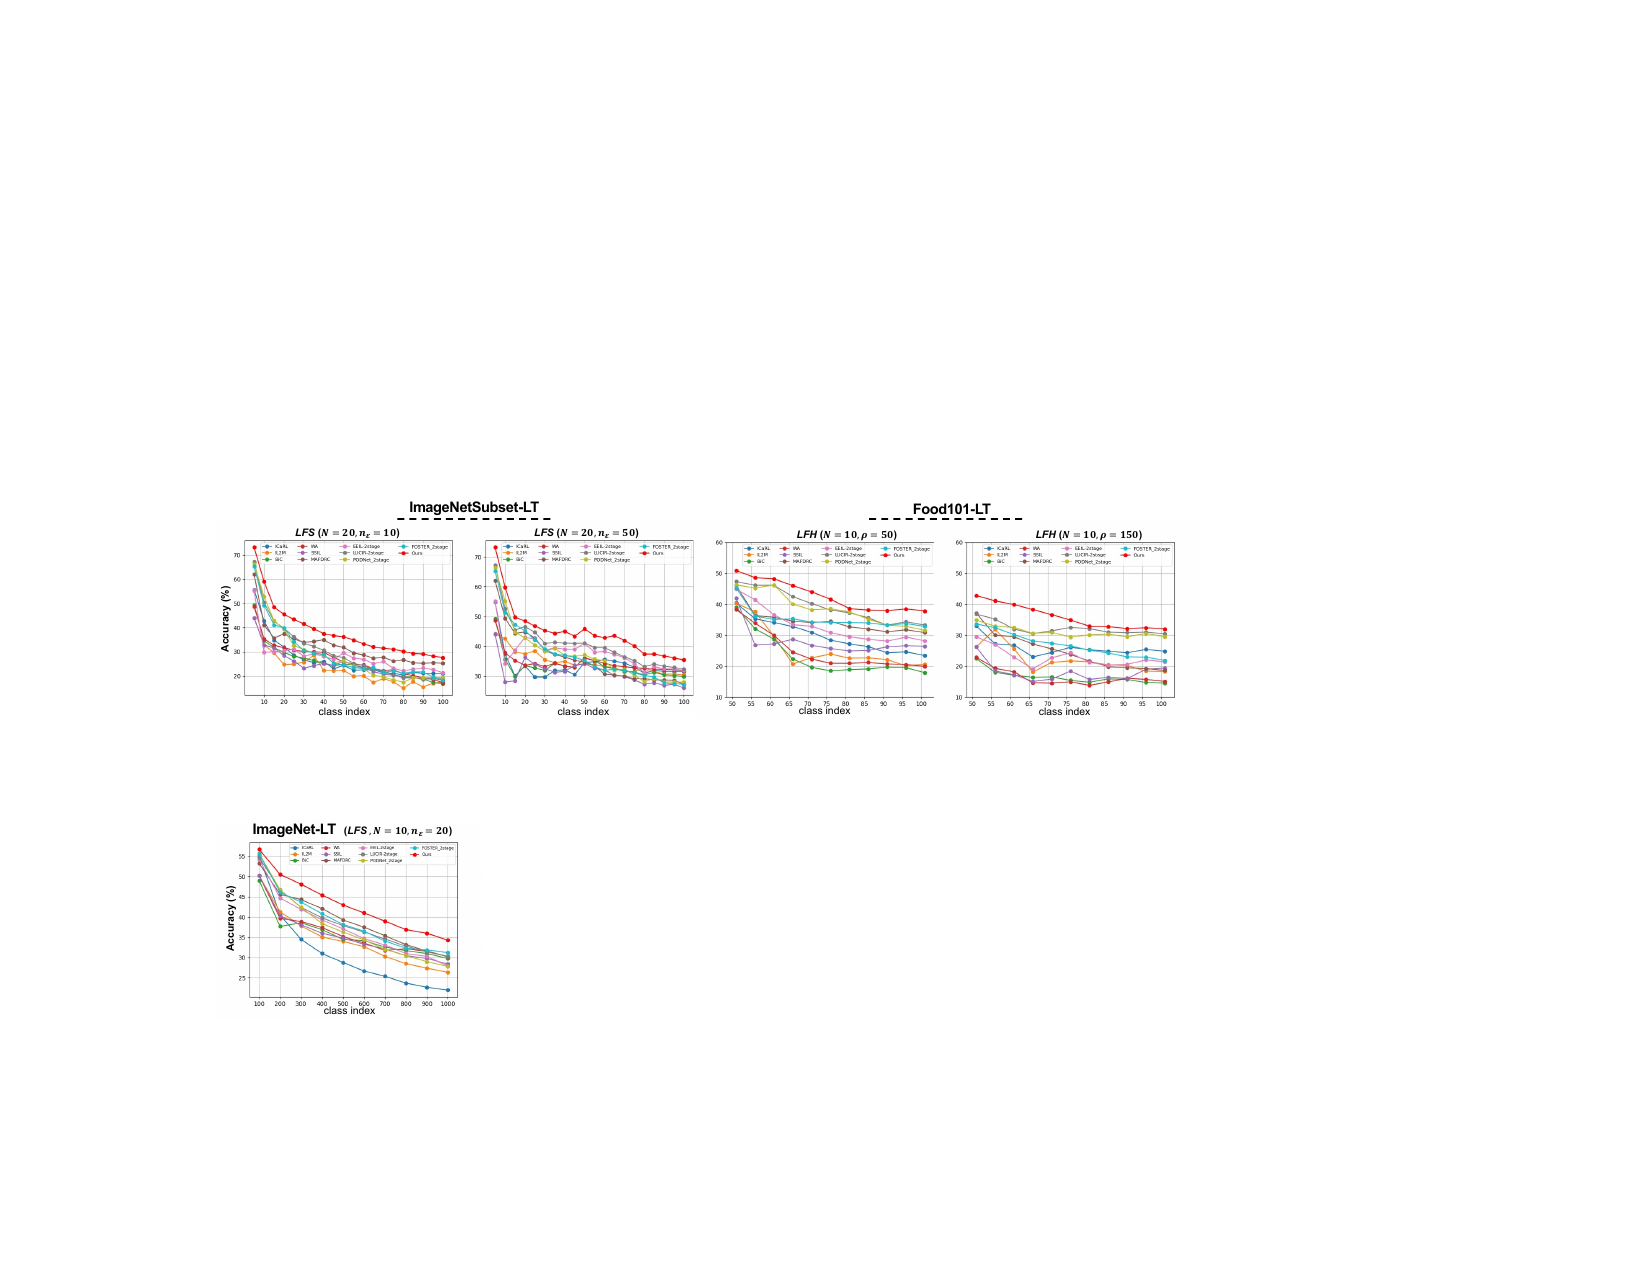}
 \caption{The classification accuracy (\%) on test data belonging to all classes seen so far at each incremental step on ImageNet-LT with imbalance factor $\rho = 100$. }
  \label{fig:imgnet-1000}
\end{center}
\end{figure}
% ----------------------

% \textbf{CIL Experiment}
% In this part, I will first illustrate the datasets such as how many train/test images in total. What is the distribution look like (may include some figures). Then I will briefly describe each of the compared methods. 

\section{Additional Experimental Results}
\label{supplsec: results}
In this part, we first present additional experimental results under imbalanced CIL and then show the effectiveness of our proposed gradient reweighting method even in conventional CIL with balanced data distribution. All the experiment setting follows the same implementation setups in Section~\ref{subsec: exp setup}.

\begin{table*}[t!]
    \centering
    \scalebox{1}{
    \begin{tabular}{|c|c|c|c|c|c|c|c|c|c|c|c|}
    \hline
        \multicolumn{1}{|c|}{Hyper-parameter $\gamma$} & 0 & 0.5 & 1.0 &  1.5 & 2.0 & 2.5 &  3.0 & 4.0 & 5.0 & 10.0 \\
        \hline
        CIFAR100-LT (\textit{LFH}, $N=10$)& 37.15 & 38.61 & 39.11 & \textbf{39.54} & 39.27 & 38.36 & 37.83 & 37.40 & 37.43 & 37.45\\
        \hline
        ImageNetSubset-LT (\textit{LFS}, $N=20$) & 39.87 & 40.63 & 40.79 & 40.87 & 41.03 & 41.14 & \textbf{41.23} & 40.36 & 40.07 & 38.18\\
        \hline
    \end{tabular}
    }
        \caption{Results of average accuracy of our proposed method by tuning hyper-parameter $\gamma \in [0,10]$ with fixed $\lambda_b = 1$. }
    \label{tab:results_gamma}
\end{table*}

\begin{table*}[t!]
    \centering
    \scalebox{1}{
    \begin{tabular}{|c|c|c|c|c|c|c|c|c|}
    \hline
        \multicolumn{1}{|c|}{Hyper-parameter $\lambda_b$} & 0.1 & 0.5 & 1.0 &  2.0 & 3.0 & 4.0 &  5.0 \\
        \hline
        CIFAR100-LT (\textit{LFH}, $N=10$) & 37.54 & \textbf{39.18} & 39.11 & 32.79 & 27.59 & 25.25 & 21.82 \\
        \hline
        ImageNetSubset-LT (\textit{LFS}, $N=20$) & 40.37 & \textbf{41.06} & 40.79 & 37.12 & 35.00 & 32.21 & 28.47\\
        \hline
    \end{tabular}
    }
        \caption{Results of average accuracy of our proposed method by tuning hyper-parameter $\lambda_b \in [0.1, 5]$ with fixed $\gamma = 1$. }
    \label{tab:results_lambda}
\end{table*}

% results for balanced convention CIL -------------------------
\begin{table*}[t!]
    \centering
    \scalebox{1.}{
    \begin{tabular}{lcccccccc}
        \hline
          \multicolumn{1}{c}{Datasets} &\multicolumn{4}{c}{\textbf{CIFAR100}} & \multicolumn{4}{c}{\textbf{ ImageNet-Subset}} \\
          
          \multicolumn{1}{c}{Evaluation protocol}  & \multicolumn{2}{c}{\textit{LFS}} & \multicolumn{2}{c}{\textit{LFH}} & \multicolumn{2}{c}{\textit{LFS}} & \multicolumn{2}{c}{\textit{LFH}}\\
          \cdashline{2-9}
          \multicolumn{1}{c}{Total tasks $N$}  & \multicolumn{2}{c}{20} & \multicolumn{2}{c}{10} & \multicolumn{2}{c}{20} & \multicolumn{2}{c}{10} \\

        \cdashline{2-9}
          \multicolumn{1}{c}{Exemplar Setup}  & GM & FM & GM & FM & GM & FM & GM & FM\\
         \hline
        iCaRL~\cite{ICARL}& 42.23 & 52.88 & 47.69 & 47.11 & 50.48 & 56.28 & 60.85 & 61.64\\
        EEIL~\cite{EEIL} & 48.39 & 59.95 & 51.65 & 54.35 & 43.20 & 54.20 & 53.05 & 56.75\\
        IL2M~\cite{dualmemory}& 48.93 & 59.12 & 51.49 & 54.75 & 44.23 & 53.31 & 51.47 & 55.06  \\
        BiC~\cite{BiC} & 52.12 & 57.47 & 33.56 & 48.55 & 51.68 & 61.27 & 58.57 & 62.32 \\
        WA~\cite{mainatining} & 51.28 & 56.73 & 35.62 & 49.13 & 49.87 & 62.94 & 56.95 & 61.82 \\
        SSIL~\cite{SSIL} & 50.84 & 57.66 & 43.52 & 47.58 & 48.74 & 58.29 & 59.30 & 59.35\\
        LUCIR~\cite{rebalancing} &  49.09 & 58.29 & 59.25 & 59.37 & 46.88 & 56.01 & 62.56 & 64.18\\
        PODNet~\cite{douillard2020podnet} & 45.45 & 53.92 & \textbf{\red{60.50}} & 61.66 & 38.33 & 49.28 & 61.41 & 63.99\\
        FOSTER~\cite{foster} & 51.90 & 63.37 & \textbf{\blue{59.54}} & \textbf{\blue{67.02}} & \textbf{\blue{56.79}} & 69.42& \textbf{\blue{63.82}}& \textbf{\blue{66.25}}\\
        MAFDRC~\cite{MAFDRC} & \textbf{\blue{52.83}} & \textbf{\red{65.68}} & 58.44 & 66.21 & 54.63 & \textbf{\red{70.18}}& 62.13& 65.47\\
          \hline
        Ours & \textbf{\red{54.30}} & \textbf{\blue{64.03}} & 59.31 & \textbf{\red{68.70}} & \textbf{\red{59.32}} & \textbf{\blue{69.56}} & \textbf{\red{67.32}} & \textbf{\red{67.20}}\\
        \hline
    \end{tabular}
    }
        \caption{Results of average accuracy for conventional CIL on original CIFAR100 and ImageNet-Subset with fixed memory (FM) budget $\mathcal{B} = 2,000$ and growing memory (GM) budget $n_\varepsilon = 20$. \textbf{\red{Best}} and \textbf{\blue{Second Best}} results are marked.}
    \label{tab:results_balanced}
\end{table*}
%-----------------------

\subsection{Results for Imbalanced CIL}
\label{subsec-supple:imbalanced CIL}
% We include the results for (i) ImageNet-LT with 1,000 classes, (ii) ordered CIL case as introduced in~\cite{liu2022long}, (iii) the fixed memory setup as described earlier in Section~\ref{subsec-supple:exemplarselection}, and (iv) tuning hyper-parameters $\gamma, \lambda_b$. 

\noindent \textbf{Results on ImageNet-LT with 1,000 classes:} We evaluate our method on large-scale datasets by constructing ImageNet-LT with 1,000 classes from ImageNet~\cite{IMAGENET1000} using imbalance factor $\rho = 100$. The experimental results are shown in Figure~\ref{fig:imgnet-1000}. Notably, even in the context of this extensive dataset, our method outperformed existing approaches at each incremental learning phase, demonstrating its efficacy in handling large-scale data in the real world. 

\noindent \textbf{Results with Ordered Long-Tailed CIL:} In accordance with~\cite{liu2022long}, we implemented Ordered Long-Tailed CIL where the learning process begins with the most frequent classes (with most training samples) and progresses towards the least frequent ones (with least training samples). This scenario is aligned with many realistic applications where learning typically starts with available common classes and gradually shifts to more challenging samples. The results on CIFAR100-LT and ImageNetSubset-LT with imbalance factor $\rho = 100$ are summarized in Table~\ref{tab:results_ordered}. We observed the results in ordered cases are typically better than the results in shuffled cases as shown in Table~\ref{tab:results_all}, which can be attributed to the significant reduction of intra-class imbalance issue in this scenario. Despite this variation in learning conditions, our method consistently demonstrated promising results, outperforming existing approaches in both ordered and shuffled long-tailed CIL without requiring the additional training stage.  

\noindent \textbf{Results with Fixed Memory Budget:} As described in Section~\ref{subsec-supple:exemplarselection}, we consider a variant of fixed memory budget $\mathcal{B}$. The results on CIFAR100-LT and ImageNetSubset-LT with imbalance factor $\rho=100$ and $\mathcal{B}\in\{500, 1000\}$ are visualized in Figure~\ref{fig:fixedmemory}. Together with the results shown in Figure~\ref{fig:results_all}, we demonstrate the adaptability of our method under both exemplar setups to achieve the best performance at each incremental learning phase. However, as illustrated in Section~\ref{subsec-supple:exemplarselection}, while the total buffer size $\mathcal{B}$ is bounded, the imbalanced CIL under a fixed memory budget usually introduces a more pronounced class imbalance issue within the exemplar set. Addressing this challenge remains a crucial area for future algorithm development. 

\noindent \textbf{Tuning Hyparameters:} As illustrated in Section~\ref{sec:method}, we introduced two hyper-parameters in this work including (i) $\gamma$ to control the magnitude of attenuation factor as in Equation~\ref{eq:ri}, and (ii) $\lambda_b$ to control the influence of knowledge distillation in the integrated objective as in Equation~\ref{eq: z}. As detailed in the experimental setup in Section~\ref{subsec: exp setup}, we use $\gamma = 1$ and $\lambda_b = 1$ for simplicity on all experiments to show the effectiveness of our method even without hyper-parameter tuning. In this part, we demonstrate that tuning these two hyper-parameters can achieve better performance. The results by tuning $\gamma$ and $\lambda_b$ are summarized in Table~\ref{tab:results_gamma} and Table~\ref{tab:results_lambda}, respectively. For $\gamma$, we observed that a moderate increment from $\gamma = 0$ gradually increases performance while a large $\gamma$ results in performance degradation. This observation is aligned with our findings as in Section~\ref{subsec: inter-phase} where the model could under-fit on new classes without $\gamma$ as the new classes receive less attention, and using large $\gamma$ will conversely result in prediction bias towards new classes due to the inter-class imbalance issue in CIL. Similarly, as $\lambda_b$ becomes larger, there is a sharp decrease in accuracy since the overly dominant knowledge distillation component in the integrated objective function can obstruct the effective learning of new classes. These observations highlight the adaptability of our method to achieve potential improvements to accommodate various applications in the real world.

% I will include additional experimental results for (1) ImageNet with 1,000 classes. (2) Ordered case (in main paper we use shuffled case) (3) the results for fixed memory, and (4) how the performance change by varying the hyper-parameters $\gamma$, $\lambda_b$ as introduced in Section~\ref{subsec: inter-phase}. 

% \subsection{Results for Imbalanced CIL in Online Scenario} (optional)
% I want to show our method is also applicable in online scenario and compared with existing methods (similar as in Sid's paper results)

\subsection{Results for Conventional CIL}
\label{subsec-supple: conventional CIL}
In this part, we highlight the effectiveness of our proposed method even under the Conventional CIL setting with class-balanced data distribution, where only the inter-phase imbalance issue is present. The results on CIFAR-100 and ImageNetSubset are summarized in Table~\ref{tab:results_balanced} where we consider both growing memory (GM) with $n_\varepsilon = 20$ and fixed memory (FM) with $\mathcal{B}=2,000$. Our method achieved promising performance across both datasets and memory setups. Notably, in the ImageNetSubset evaluations, our method significantly outperformed existing approaches under the GM setup, where the inter-phase imbalance issue presents a more substantial challenge. Additionally, we achieved promising performance under FM setup on CIFAR-100 and ImageNetSubset datasets under both evaluation protocols with varied incremental phases. These results further demonstrate the adaptability and effectiveness of our proposed method in a broader CIL context with various learning conditions.

\subsection{Long-tailed Recognition}
\label{subsec-supple: long-tail}
In this section, we evaluate our gredient reweighting for its efficacy in solving the imbalanced image classification beyond CIL by conducting comparative analyses with established methods in long-tailed recognition. We denote our regularized softmax output illustrated in Section~\ref{subsec: intra-phase} as RS. Specifically, we train a ResNet-32 to classify the 100 classes in CIFAR100-LT with various imbalance factor $\rho \in \{10, 50, 100\}$ following the training protocol as in~\cite{cui2019class}. The results are summarized in Table~\ref{tab:results_lt}. Our method shows competitive performance even without the use of regularized softmax output. Upon integrating the regularized softmax output, which further balances the learning process, we consistently achieve improved classification accuracy and outperform existing methods.

\begin{table}[t]
    \centering
    \scalebox{.83}{
    \begin{tabular}{lccc}
        \hline
           &\multicolumn{3}{c}{\textbf{CIFAR100-LT}} \\
           & $\rho = 100$ &  $\rho = 50$ &  $\rho = 10$ \\
        %    & \multicolumn{2}{c}{\textit{LFS}} & \multicolumn{2}{c}{\textit{LFH}} & \multicolumn{2}{c}{\textit{LFS}} & \multicolumn{2}{c}{\textit{LFH}} & \multicolumn{2}{c}{\textit{LFS}} & \multicolumn{2}{c}{\textit{LFH}}\\
        % \cdashline{2-13}
          % \multicolumn{1}{c}{Total tasks $N$}  & 10 & 20 & 5 & 10 & 10 & 20 & 5 & 10 & 10 & 20 & 5 & 10\\
         \hline
        % Baseline & 38.29 & 42.54 & 54.87 \\
        ROS~\cite{ROS} & 36.32 & 41.28 & 55.12 \\
        Focal Loss~\cite{FocalLoss} & 38.91 & 43.26 & 55.08 \\
        LDAM~\cite{LDAM} & 40.82 & 45.68 & 57.32\\
        CB Loss~\cite{cui2019class} & 39.62 & 46.29 & 57.29\\
        IB Loss~\cite{IBLoss} & 43.62 & 46.80 & 58.01\\
        BS Loss~\cite{BSLoss} & 44.12 & 49.25 & 59.38 \\
        % EQL~\cite{tan2020equalizationv1}  & 42.96 & 47.83 & 57.24  \\
        EQL v2~\cite{tan2021equalizationv2} & 43.81 & 48.25 & 57.06 \\
        CMO~\cite{CMO}  & 43.54 & 47.92 & 58.97 \\
          \hline
        Ours \textit{w/o} RS & 43.84 & 47.39 & 57.95  \\
        Ours  & \textbf{45.27} & \textbf{49.02} & \textbf{60.71}  \\
        \hline
    \end{tabular}
    }
        \vspace{-2ex}\caption{Long-tailed recognition accuracy (\%) on CIFAR100-LT with imbalance factor $\rho \in \{100, 50, 10$\}}
            \label{tab:results_lt}
        \vspace{-0.2cm}
\end{table}

\subsection{Computation and Memory Efficiency}
\label{subsec-supple: efficiency test}

Our framework employs a compact vector, denoted as $\Phi$, for the computation of accumulated gradients. To elucidate the storage usage, we consider the following detailed analysis. Assuming $\Phi$ comprises $N$ elements, where each element is a floating-point number represented using 32 bits (or 4 bytes) of memory, the total storage requirement for $\Phi$ can be quantified using the equation:

\begin{equation}
\text{Storage}_{\Phi} = N \times 4  \text{(bytes)}
\end{equation}

For CIL, $N$ refers to the number of classes seen so far. Consequently, for datasets with $100$ classes such as CIFAR100 or ImageNetSubset, $N = 100$ at the last incremental learning phase, rendering the storage used by $\Phi$ as follows:

\begin{equation}
\text{Storage}_{\Phi} = 100 \times 4  = 400  \text{(bytes)}
\end{equation}

To provide a comparative perspective on this storage efficiency, we consider the storage required by a single RGB image from the CIFAR dataset. Each CIFAR image, with a resolution of $32 \times 32$ pixels and utilizing 8 bits (or 1 byte) per pixel for each of the three RGB color channels, necessitates the following storage
\begin{equation}
\text{Storage}_{\text{CIFAR}} = 32 \times 32 \times 3  = 3072 \text{(bytes)}
\end{equation}
The ratio of storage usage can be calculated as 
\begin{equation}
\frac{\text{Storage}{\Phi}}{\text{Storage}{\text{CIFAR}}} = \frac{400}{3072} \approx 0.13
\end{equation}
Thus the total usage of storage for calculating $\Phi$ will be around $1/10$ of one single CIFAR image, while it brings significant performance improvements as shown in our experiments.  

In terms of computational efficiency, our framework is designed for end-to-end training. This integrated approach sidesteps the substantial computational overhead typically associated with decoupled training phases. For instance, existing methods such as~\cite{liu2022long} require 30 additional epochs for balanced fine-tuning. Our experimental results underscore the substantial performance enhancements achieved through our methodology. These improvements are not merely computational but also extend to the accuracy and efficiency of the training process, showing great potential for facilitating high-effiency models in real-world applications.
